# Supplementary material for: Wettability stabilizes fluid invasion into porous media via nonlocal, cooperative pore filling
Source: arXiv:1509.04423 source file (2015-09-15)
Supplement: Supplementary file 1 [file Holtzman_Supp_Mat_wettability_letter_3.pdf]

# Supplemental Material for Wettability stabilizes fluid invasion into porous media via nonlocal, cooperative pore filling

Ran Holtzman<sup>1,\*</sup> and Enrico Segre<sup>2</sup>

<sup>1</sup>*Department of Soil and Water Sciences, The Hebrew University of Jerusalem, Israel*

<sup>2</sup>*Physics Services, Weizmann Institute of Science, Israel*

Here we provide the essential details of the pore-scale model and the derivation of the dimensionless groups  $N_{ca}$  and  $N_{coop}$ , and movies showing the displacement dynamics.

## Pore-scale model of the displacement dynamics at arbitrary wettability

We present here a novel pore-scale model of immiscible fluid-fluid displacement in a disordered porous medium, with fluids of arbitrary viscosities and contact angle. A two-dimensional (2-D) heterogeneous medium is constructed by placing cylindrical solid particles on a triangular lattice with spacing  $a$ , selecting the particle diameters  $d$  from an assigned distribution; here we use uniform distribution,  $d \in [1 - \lambda, 1 + \lambda]\bar{d}$ , where  $\lambda \in (0, 1)$  represents the degree of disorder, and  $\bar{d} \lesssim a$  is the mean diameter [Fig. S1(a)]. Each particle triplet defines a pore with volume  $V$  connected to three neighboring pores by throats with aperture  $0 < 2\rho \lesssim a$ ; to avoid particle overlap we enforce  $\bar{d} < a/(1 + \lambda)$ . A triangular lattice is chosen for its simplicity, allowing only up to two menisci to invade an unfilled pore, thus capturing the essence of cooperative pore filling at minimal algorithmic complexity (e.g. avoiding the ambiguity associated with resolving a burst on a square lattice [1]).

We model the fluid-fluid interface by a sequence of circular menisci, intersecting pairs of particles at the prescribed contact angle  $\theta$ , with a curvature  $1/R = \Delta p/\gamma$  supporting a capillary pressure  $\Delta p$  [Fig. S1(a)]. In our 2-D model, the meaning of  $R$  depends on the model geometry. For elongated particles with height (measured into the page) much larger than diameter,  $h \gg d$ , the meniscus geometry can be assumed 2-D since the in-plane curvature is much larger than the out-of-plane curvature,  $R_{in} \ll R_{out}$ , providing  $R = 1/(R_{in}^{-1} + R_{out}^{-1}) \approx R_{in}$ . Otherwise, if  $h \approx d$  and  $h \gtrsim 2\rho$ , the meniscus can be approximated as hemispherical, with  $R_{in} \lesssim R_{out}$  and  $R \approx 2R_{in}$ . Here we consider the former,  $R = R_{in}$ .

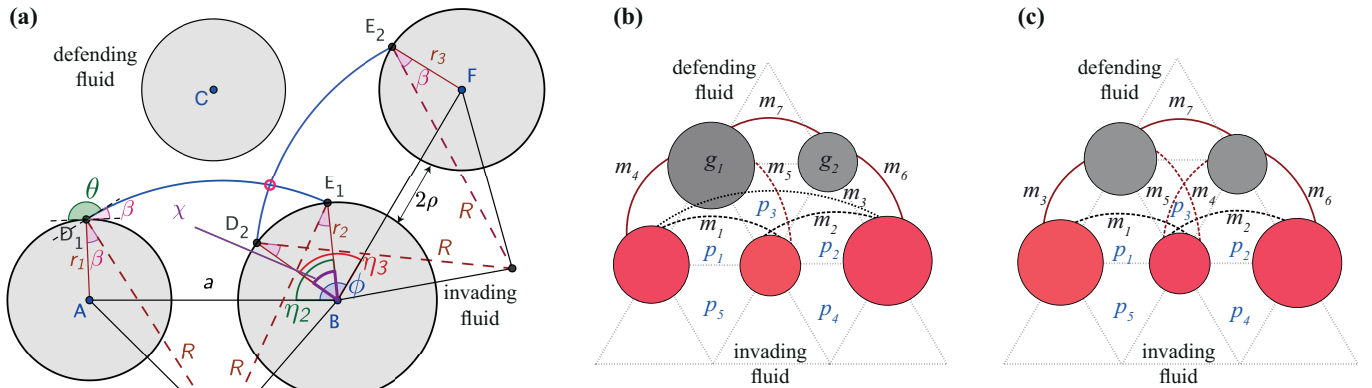

Figure S1. (color online). Geometrical details of our model. (a) Each meniscus (in blue) intersects a pair of particles at the prescribed contact angle  $\theta$  and has a curvature  $1/R$  (the complementary angle,  $\beta = 180 - \theta$  is marked in pink). Overlap precedes burst (while  $R > R_c$ ) when  $\chi = \phi - \eta_2 - \eta_3 < 0$  (in purple), see text. Once pore invasion ends, we update the meniscus configuration, as shown in (b) and (c) for two cases of overlap at  $\phi = 180^\circ$ , complicated due to a succession of events (allowing demonstration of other, simpler cases). Two menisci  $m_1$  and  $m_2$  separating invaded ( $\Phi = 1$ ) pores  $p_4$  and  $p_5$  and non-invaded ( $\Phi = 0$ ) pores  $p_1$  and  $p_2$  are destabilized by overlap. The interface progression is determined by fusing  $m_1$  and  $m_2$  into a single arc,  $m_3$ . In (b),  $m_3$  is further destabilized by touching grain  $g_1$ , causing the filling of pore  $p_1$  (also of  $p_2$  if  $g_2$  was touched); once filled, the interface configuration is updated by replacing  $m_3$  with two new arcs,  $m_4$  and  $m_5$ . Here,  $m_5$  is further destabilized by overlap with  $m_2$  (at  $\phi = 120^\circ$ ); they are replaced by a fused arc (not shown) destabilized by touching grain  $g_2$ , causing filling of both  $p_2$  and  $p_3$ . The final stable configuration is obtained by replacing  $m_2$  and  $m_5$  with  $m_6$  and  $m_7$ . In (c), the fused arc of curvature  $1/R$  is geometrically inadmissible, causing advancement of both  $m_1$  and  $m_2$  to fill  $p_1$  and  $p_2$  (at different rates, depending on the local fluxes), after which they are replaced with  $m_3$ – $m_7$ . Arcs  $m_4$  and  $m_5$  are immediately destabilized by overlap ( $\phi = 60^\circ$ ) that causes filling of  $p_3$ , and eventually replaced by  $m_7$ .

Menisci are tested for three types of instabilities [1]: (1) *burst* (Haines jump), when the curvature exceeds a threshold set by local geometry; (2) *touch*, when a meniscus intersects a third, downstream particle; and (3) *overlap* of adjacent menisci, destabilizing each other (Fig. 1 in the Letter). While a meniscus can become unstable according to several criteria simultaneously, the order by which the instabilities are treated was found to have a minor effect on our results; similar findings were reported by [2] for the model in [1].

Destabilized menisci incipiently invade the downstream pores. As discussed in details below, our model captures the crucial spatiotemporal nonlocal nature of pore invasion, by evaluating the rate of pore filling from the viscous resistance in the fluids. The front is defined as the set of throats (menisci connecting particle pairs) separating fully-invaded pores ( $\Phi = 1$ ) from accessible, non-invaded ( $\Phi = 0$ ) or partially-filled ( $0 < \Phi < 1$ ) pores, where  $\Phi$  is the filling status. Accessibility is determined from the topological connection with the outer boundary, so that trapped inclusions of defending fluid can form and persist. Meniscus stability and rate of advancement are set by the local pressure difference across the two pores it separates, and the aforementioned geometrical conditions.

We evaluate the pore pressures and consequent filling rates by resolving the flow throughout the network of contiguous pores occupied by same fluid and through throats with an unstable, advancing menisci (neglecting changes in fluid volume due to small interfacial advancement in stable menisci). Flow is evaluated from the conservation of mass for an incompressible fluid in each pore (Kirchhoff's law)  $\sum_j q_j = 0$ , summing over all connected pores  $j$ . The volumetric flow rate into a pore from its neighbor  $j$  is evaluated by assuming Stokes flow,  $q_j = C_j \nabla p_j$ , where  $C \sim \rho^4 / \mu_{\text{eff}}$  is the conductance [Fig. S1(a)]. The gradient  $\nabla p_j = (p_j - p) / \Delta x_j$  is evaluated from the pressure difference between the two pores (the capillary pressure if they contain different fluids), assuming that most of the resistance occurs in the pore constriction, over a distance  $\Delta x_j = \rho_j$ . Using an effective viscosity,  $\mu_{\text{eff}} = (\mu_i - \mu_d) \Phi + \mu_d$ , where  $\mu_d$  and  $\mu_i$  are the defending and invading fluid viscosities, allows us to use  $q$  for fluid flow between two pores containing the same fluid as well as pore filling [3]. The interpore conductance  $C$  therefore depends on the connecting throat aperture,  $\rho$ , as well as the filling status of the downstream pore,  $\Phi$ . Front readjustments are incorporated by allowing partially-filled pores which can also re-empty upon reversal of the direction of meniscus advancement ( $p > p_j$  and  $q_j < 0$ ).

We track the displacement progression using a staggered, adaptive Euler time-stepping: at each time step we (a) locate the position of the front from the filling status  $\Phi$ , and define the flow network; (b) evaluate the pore pressure  $p$  and flow rate  $q$ ; (c) check for new meniscus instabilities and update the flow network accordingly; and (d) update the filling status of each invaded pore (downstream of unstable menisci) by  $\Phi(t + \Delta t) = \Phi(t) + q^{\text{inv}}(t) \Delta t / V$ , where  $q^{\text{inv}} = \sum_u q_u$  is the invading fluid inflow (summing over all throats with unstable menisci). The timestep  $\Delta t$  is chosen adaptively so that only a fraction a pore volume is filled; this allows us to capture the disparate timescales of pore filling and bulk flow [4, 5], a major computational challenge [6, 7]. When pore invasion ends ( $\Phi = 1$ ), the new interface configuration is resolved by replacing the unstable arcs with new ones that touch the upstream particle, as shown in Fig. S1(b–c) for overlap at  $\phi = 180^\circ$ , complicated due to a succession of events (therefore allowing demonstration of other, simpler cases). This description provides the nonlocal interaction between menisci and the times of meniscus advancement and pore invasion in a simple, computationally efficient manner as it excludes the cumbersome explicit geometrical evaluation of the changes in fluid volume associated with curvature changes.

We enforce a constant injection rate by setting the hydraulic resistance of the injection region (a disk of size of several pores) to be orders of magnitude larger than elsewhere, and fixing a large pressure drop between the inlet and outermost (outlet) pores; this ensures a practically constant pressure gradient regardless of front position. The simulations are terminated when an outlet pore is invaded. For further details of our numerical algorithm see the attached pseudocode.

### Modeling the dynamics of fluid displacement

The intricate displacement dynamics, including interface readjustments, residual films and snapoff, contact line and contact angle dynamics, are subject of intensive research [6–9]. In particular, contact line and angle dynamics and hysteresis are highly sensitive to physical and chemical heterogeneities which are hard to characterize, requiring microscopic models up to the atomistic level [6, 9]. Here, we focus on the essential mechanisms associated with the cooperative, nonlocal interface dynamics, including the spatial nonlocal effect of pore filling on the interface configuration in other locations, and temporal effect due to the separation of timescales of pore filling and bulk flow [4, 5], by accounting for viscous dissipation in computing the pore filling rates. Consequently, our model provides the crucial effects of pressure screening [10, 11] and interface readjustments [4, 12, 13] associated with rapid interface advancement which increases the pressure of the defending fluid, thereby decreasing the capillary pressures along the front. Pressure screening occurs at high flow rates, where the entire interface is destabilized but only the tips of the most advanced fingers propagate, due to the high defending fluid pressure in the “gulfs” between the fingers. Interface readjustments are caused by rapid redistribution of the defending fluid along the invasion front together with flow of invading fluid from nearby interfacial sites, reducing the capillary pressure and causing the meniscus to recede as the local curvature decreases. This crucial mechanism explains the disparate timescales of pore filling and bulk flow, and the limitation of avalanches

(simultaneous invasion of multiple pores) sizes by suppressing further invasion until the excess pressure in the defending fluid is dissipated by flow [4, 5, 12–14].

While our model considers these crucial mechanisms, it excludes other details including film flow, snapoff, and velocity-dependence of the contact angle. This simplification is justified because these details have a smaller impact on the displacement behavior for the problem considered here, and, since the models describing them are being strongly debated [6, 8, 9], including them in our model may actually weaken our results, in addition to making computations intractable [6, 7]. Specifically, we note that film flow and snapoff have a minimal effect for the type of medium and conditions considered here: high disorder and porosity, small throat to pore size ratio, and large viscosity ratio [7, 15–17]. We also find that introducing an empiric correction in the form of a dynamic contact angle does not significantly affect our results. A noticeable difference between static and dynamic angles occurs only at the highest  $Ca$  considered here, where the angle has a minor effect, and only for small angles; at lower  $Ca$  the difference is minor, whereas at small angles the invasion is relatively insensitive to  $\theta$  (Fig. 2 in the Letter). The fact that our model predicts the experimentally-observed invasion behavior across a large range of contact angles and flow rates [18, 19] implies that it incorporates the essential mechanisms, and that details we have simplified are less important. By modeling only the most essential mechanisms in a computationally efficient manner, our model provides, for the first time, the simultaneous effects of dynamics and wettability in a large, disordered domain, overcoming a computational challenge that has restricted simulations of partially-wetting invasion to either quasi-static (e.g. [1, 20]) or small, homogenous domains [6, 7]).

### Derivation of the dimensionless numbers by scaling analysis

#### *Characteristic critical burst curvature*

Considering a positive curvature (higher invading fluid pressure), we find the bursting threshold,  $R = R_c$ , from the geometrical conditions for the existence of a stable arc intersecting the particles at an angle  $\theta$  [1]:

$$R_c = (\alpha_1 + a\sqrt{\alpha_2}) / 2\alpha_3 \quad (S1)$$

where

$$\begin{aligned} \alpha_1 &= r_1 (r_1^2 - r_2^2 - a^2) \cos \theta - r_2 (r_1^2 - r_2^2 + a^2) \cos \theta \\ \alpha_2 &= a^2 (a^2 - 2r_1^2 - 2r_2^2) + (r_1^2 - r_2^2)^2 + 4r_1 r_2 (a^2 - r_1^2 - r_2^2) \cos^2 \theta + 2(2r_1 r_2 \cos \theta)^2 \\ \alpha_3 &= a^2 - [(r_1 - r_2) \cos \theta]^2. \end{aligned}$$

The critical curvature used in the derivation of  $N_{ca}$  and  $N_{coop}$  is obtained by replacing  $r_1, r_2$  with the normalized mean diameter  $\tilde{l} = \bar{d}/a$ ,

$$R_c = \frac{a}{2} \left( \sqrt{1 - \tilde{l}^2 \sin^2 \theta} - \tilde{l} \cos \theta \right). \quad (S2)$$

#### *Geometrical conditions for overlap preceding burst*

Overlap of menisci is expressed by the geometrical condition  $\chi < 0^\circ$  or  $\chi > 360^\circ$ , where  $\chi = \phi - \eta_2 - \eta_3$  and  $\phi = \angle ABF$  is the local front shape, which for our triangular lattice can take one of five values,  $\phi = n \cdot 60^\circ$  with  $n = 1 \div 5$  [Fig. S1(a)]. In our simulations, disorder may cause the curvatures of the two overlapping menisci to differ, therefore we consider the general case of  $\eta_2 \neq \eta_3$ . Here, to derive  $N_{coop}$  we consider a homogenous lattice (uniform  $r$ ) and similar curvatures  $R$  in the two arcs, providing  $\eta_2 = \eta_3 = \eta$ , where

$$\eta = \cos^{-1} \left( \frac{r + R \cos \theta}{\sqrt{R^2 + r^2 + 2Rr \cos \theta}} \right). \quad (S3)$$

Considering only the most common case of overlap,  $\chi < 0$ , and noting that  $\chi$  is a monotonically decreasing function of  $R$  for all values of  $\phi, r$  and  $\theta$ , if  $\chi < 0$  at the critical burst curvature  $R_c$  [Eq. (S2)] then  $\chi = 0$  for some lower pressure  $R > R_c$ , implying that an overlap would occur before burst. The geometrical condition for overlap at *exactly* the bursting curvature,  $\chi = \phi - \eta_2 - \eta_3 = 0$ , is found by substituting  $R = R_c$  in Eq. (S3),

$$\eta = \cos^{-1} \left[ \frac{r [1 - \cos(2\theta)] + \cos \theta \sqrt{a^2 - 4r^2 (1 + \cos \theta)}}{a} \right]. \quad (S4)$$

Finally, we define the “Cooperative number” as

$$N_{\text{coop}} = \cos \frac{\phi}{2} - \tilde{l} \sin^2 \theta + \cos \theta \sqrt{1 - \tilde{l}^2 \sin^2 \theta}, \quad (\text{S5})$$

such that  $N_{\text{coop}} = 0$  coincides with the geometrical condition  $\chi = 0$  (using the invertibility of the cosine within  $0^\circ \leq \eta \leq 180^\circ$ ), and  $N_{\text{coop}} > 0$  implies overlap *preceding* burst. We stress that the local front shape  $\phi$  varies in time and space, and that the condition for overlap preceding burst  $\chi = 0$  was derived here for a homogenous system with equal curvatures of the overlapping arcs; therefore, in a disordered system not all pores will be invaded by the same instability at a given  $N_{\text{coop}}$ . Since the overall pattern is a consequence of many invasion events,  $N_{\text{coop}}$  should be considered in a *statistical* sense: a larger  $N_{\text{coop}}$  value implies a higher fraction of overlaps, and therefore a more compact pattern. Here we computed  $N_{\text{coop}}$  using  $\phi = 120^\circ$  [two menisci advancing into two adjacent pores, Fig. S1(a)] which we found to be most representative for our system [21].

### Videos showing the invasion dynamics

The dynamics of fluid invasion leading to the emergence of the patterns in the different regimes (boxed in red in Fig. 2(d) in the Letter) is demonstrated by videos. Invaded pores appear in gray, highlighting in red the active front (pores currently invaded). The injection region is marked by a black circle.

1. Video 1a ( $\text{Ca} = 3.2 \cdot 10^{-3}$ ,  $\theta = 5^\circ$ ) and 1b ( $\text{Ca} = 3.2 \cdot 10^{-3}$ ,  $\theta = 120^\circ$ ): *Viscous fingering*—continuous advancement of individual fingers towards the outlet, splitting at their tips. The final pattern is radial with thin fingers and highly irregular interfaces, exhibiting little trapping of the defending fluid. Occurring at high injection rates, irrespective of  $\theta$ .
2. Video 2 ( $\text{Ca} = 1.3 \cdot 10^{-5}$ ,  $\theta = 5^\circ$ ): *Capillary fingering*—intermittent propagation of different parts of the interface, leading to a asymmetrical pattern with a fractal interface and multiple trapped clusters. Occurring at slow drainage (low  $\text{Ca}$  and  $\theta$ ).
3. Video 3 ( $\text{Ca} = 1.3 \cdot 10^{-5}$ ,  $\theta = 120^\circ$ ): *Compact displacement*—simultaneous advancement of large parts of the interface, providing continuous, radial growth of a dense pattern with a stable, smooth interface. Occurring at slow imbibition (low  $\text{Ca}$ , high  $\theta$ ).

---

\* holtzman.ran@mail.huji.ac.il

- [1] M. Cieplak and M. O. Robbins, Phys. Rev. B **41**, 11508 (1990).
- [2] I. Hecht and H. Taitelbaum, Phys. Rev. E **70**, 046307 (2004).
- [3] R. Lenormand, E. Touboul, and C. Zarcone, J. Fluid Mech. **189**, 165 (1988).
- [4] R. T. Armstrong and S. Berg, Phys. Rev. E **88**, 043010 (2013).
- [5] S. Berg, H. Ott, S. A. Klapp, A. Schwing, R. Neiteler, N. Brussee, A. Makurat, L. Leu, F. Enzmann, J.-O. Schwarz, M. Kersten, S. Irvine, and M. Stampanoni, Proc. Natl. Acad. Sci. U.S.A. **110**, 3755 (2013).
- [6] P. Meakin and A. M. Tartakovsky, Rev. Geophys. **47**, RG3002 (2009).
- [7] V. Joekar-Niasar and S. M. Hassanizadeh, Crit. Rev. Environ. Sci. Technol. **42**, 1895 (2012).
- [8] M. Alava, M. Dubé, and M. Rost, Adv. Phys. **53**, 83 (2004).
- [9] D. Bonn, J. Eggers, J. Indekeu, J. Meunier, and E. Rolley, Rev. Mod. Phys. **81**, 739 (2009).
- [10] L. Niemeyer, L. Pietronero, and H. J. Wismann, Phys. Rev. Lett. **52**, 1033 (1984).
- [11] G. Løvøll, Y. Méheust, R. Toussaint, J. Schmittbuhl, and K. J. Måløy, Phys. Rev. E **70**, 026301 (2004).
- [12] K. J. Måløy, L. Furuberg, J. Feder, and T. Jøssang, Phys. Rev. Lett. **68**, 2161 (1992).
- [13] L. Furuberg, K. J. Måløy, and J. Feder, Phys. Rev. E **53**, 966 (1996).
- [14] L. Xu, S. Davies, A. B. Schofield, and D. A. Weitz, Phys. Rev. Lett. **101**, 094502 (2008).
- [15] R. Lenormand, J. Phys. Condens. Matter **2**, SA79 (1990).
- [16] M. S. Al-Gharbi and M. J. Blunt, Phys. Rev. E **71**, 016308 (2005).
- [17] V. Joekar-Niasar, S. M. Hassanizadeh, L. J. Pyrak-Nolte, and C. Berentsen, Water Resour. Res. **45**, 1 (2009).
- [18] J. P. Stokes, D. A. Weitz, J. P. Gollub, A. Dougherty, M. O. Robbins, P. M. Chaikin, and H. M. Lindsay, Phys. Rev. Lett. **57**, 1718 (1986).
- [19] M. Trojer, M. L. Szulcowski, and R. Juanes, Phys. Rev. Appl. **3**, 054008 (2015).
- [20] M. Cieplak and M. O. Robbins, Phys. Rev. Lett. **60** (1988).
- [21] The representative value of  $\phi$  may change with the medium geometry, for instance with porosity, mean particle size and its variance.
